# Supplementary material for: Learning Syntax Without Planting Trees: Understanding Hierarchical Generalization in Transformers
Source: arXiv:2404.16367 source file (2025-03-16)
Supplement: Supplementary file 1 [file appendix.tex]

\appendix
\section{Model Architectures}
\label{app:architectures}
We experiment with a set of neural autoregressive sequence models that model the generative process of a sequence via $ \Pi_{i=1}^T p_{m}\left(\vx_{i+1} \mid \vx_{1:i}\right)$. We characterize each model with three common consecutive modules: (i) an \textbf{embedding layer} that maps input tokens to vectors, (ii) a stack of \textbf{backbone layers}, (iii) and an \textbf{output projection} layer that maps the final outputs from the backbone to the distribution over the token space.
\begin{equation}
p_{m}\left(\vx_{i+1} \mid \vx_{1:i}\right) = \softmax{\left(m_{\textrm{output}} \circ m_{\textrm{backbone}} \circ m_{\textrm{embed}}\left(\vx_{1:i}\right)\right)}
\end{equation}
Collectively, the three modules form a mapping from one-hot vectors to pre-softmax logits, i.e., $\{0, 1\}^{T \times |V|} \rightarrow \R^{T \times |V|}$ where $T$ denotes the sequence length, $|V|$ denotes the vocabulary size.

\paragraph{Embedding Layer ($m_{\textrm{embed}}$)}
The embedding layer is a single projection matrix which converts one-hot input vectors to dense vectors: 
\begin{equation}
    m_{\textrm{embed}}(\vx) = \mW_{e}\,\vx. 
\end{equation}
In almost all models, the positional information need not be incorporated in the embedding layer. It is either explicitly added as the rotary positional embeddings (Rope,~\citet{su2024roformer}) in the attention layer, or implicitly handled in the recurrence/convolution form of models.  The only exception is the original Transformer with multi-head attention, where positional information is added as learnt positional embeddings:
\begin{equation}
    m_{\textrm{embed}}(\vx)_i = \mW_{e}\,\vx_i + \mW_{p}\,\vi,
\end{equation}
where $\vi$ is one-hot representation of the time-step $t$. We use the original Transformer in our synthetic experiments, and use the improved Transformer with Rope in our language modelling experiments on real data.

\paragraph{Backbone Layers ($m^{(l)}_{\textrm{backbone}}$)}
Each backbone layer updates the previous layer's hidden outputs ($\vh^{(l-1)}$) in two sequential steps. First, a \textbf{token mixer} that models the token-level interactions. Effectively,  it can be any \emph{causal} network mapping  hidden states of previous tokens to a new hidden state for the current token:
\begin{equation}
\va^{(l)} = m^{(l)}_{\textrm{mixer}}\left(\vh^{(l-1)}\right),
\end{equation}
where $m^{(l)}_{\textrm{mixer}}\left(\vh^{(l-1)}\right)_i = m^{(l)}_{\textrm{mixer}}\left(\vh^{(l-1)}_{1:i}\right)_t$.
Then, a \textbf{feed-forward} network, $m^{(l)}_{\textrm{FF}}$, applied to the final outputs of the layer with a residual connection:
\begin{equation}
m^{(l)}_{\textrm{backbone}}(\vh^{(l-1)})= m^{(l)}_{\textrm{FF}}\left(\va^{(l)} \right) + \va^{(l)}.
\end{equation}
or alternatively in a gated-linear unit (GAU,~\citet{hua2022transformer}) structure:
\begin{equation}
m^{(l)}_{\textrm{backbone}}(\vh^{(l-1)})= m^{(l)}_{\textrm{GAU}}\left(\vh^{(l-1)}, \va^{(l)}  \right) + \va^{(l)}.
\end{equation}
where $m_{\textrm{GAU}}(\vx, \vy) = \mW_3  (\mW_1 \vx) \odot (\mW_2\vy)$, and $\odot$ denotes element-wise product.~\footnote{Among all the models presented, only Mamba employs the GAU architecture.} In contrast to the token mixer, the feed-forward network is applied individually for each token, i.e., there is no token-wise interactions.

\paragraph{Output Projection ($m_{\textrm{output}}$)} The projection layer consists of a single fully-connected projection that converts the outputs of the backbone $\vh^{(L)}$ to the output space:
\begin{align}
    m_{\textrm{output}}(\vh^{(L)}) = \rmW_{o}\,\vh^{(L)}
\end{align}

In the following sections, we review the model architectures studied in this work - they share the common skeleton presented above, and mainly differ in the design of the token-mixing module $m_{\textrm{mixer}}$.~\footnote{For brevity, we omit the normalization layers which are applied before each token mixer and feed-forward layer.}. We intend to present a unified view of all models by using shared notations and equivalent forms (when possible). 

We will denote input/output of a token mixer as $\vx \in \R^{L \times d}$ and $\vy \in \R^{L \times d}$, respectively. When possible, we will present all the possible forms (i.e., attention-style form, recurrent form and convolutional form) of a model. Generally, attention-style/convolutional forms are useful for developing training schema, whereas recurrent forms are crucial for model's inference schema.

\subsection[Transformers with Self Attention]{Transformers with Self Attention \citep{vaswani2017attention}}\label{app:transformers}
Standard self-attention performs token mixing in the following way:
\begin{align}
    & \vq_i, \vk_j  = \mW_q\vx_i ,\mW_k \vx_j  \in \R^{d_k}   \\
    & \mA_{ij}  \propto \exp(\langle \vq_i, \vk_j \rangle) \in (0,1) \qquad \text{softmax attention} \\
    & \vv_j = \mW_v \vx_j \in \R^{d_v} \\
    & \vz_{i} = \sum_{j=1}^i \mA_{ij} \vv_j \in \R^{d_v} \label{eq:self-att}  \\
    & \vy_{i} = \mW_o \vz_{i} \in \R^{d}
\end{align}
where $d_k, d_v$ denote the dimension for query/key and value vectors, respectively. 
The attention scores are computed based on the pairwise dot-product between the query vector of the current token and key vectors from the context. In the multi-head attention, attention output $\vz_i$ is independently computed  in each head; all outputs are concatenated as the final attention output, which will then be fed into the output projection $\mW_o$. %

\subsection[Transformers with Linear Attention]{Transformers with Linear Attention~\citep{katharopoulos2020transformers}}\label{app:lineartransformers}

The linear attention~\citep{katharopoulos2020transformers} simplifies the standard attention by replacing $\exp(\langle \vq_i, \vk_j \rangle)$ with a kernel map $k(\vq_i, \vk_j )$ with an associative feature map (i.e., $k(\vq_i, \vk_j ) = \phi(\vq_i) \phi(\vk_j)$). In this work, we consider a simple feature map of identity function (i.e., $\phi(\vq_i) = \vq_i$), which yields surprisingly good performance for language model on real data in recent works~\citep{qin2022devil,yang2023gated}. With this feature map, the token mixing process is very similar to standard attention, except that attention scores are not normalized.%
\begin{align}
& \vq_i, \vk_j =  \mW_q\vx_i ,\mW_k \vx_j  \in \R^{d_k}  \\
& \mA_{ij} = \langle \vq_i, \vk_j \rangle \qquad \text{linear attention}   \\
& \vv_j = \mW_v \vx_j \in \R^{d_v}  \\
& \vz_{i} = \sum_{j=1}^i \mA_{ij} \vv_j \in \R^{d_v} \qquad \label{eq:self-att-linear} \\
&  \vy_{i} = \mW_o \vz_{i} \in \R^{d}
\end{align}

The linear attention has an equivalent recurrent form as follows.
\begin{align}
& \vq_i, \vk_j =  \mW_q\vx_i ,\mW_k \vx_j  \in \R^{d_k}  \\
& \rmS_{i} = \rmS_{i-1} + \vk_i^\intercal \vv_i \in \R^{d_k \times d_v} \\
&\vz_i = \vq_i^{\intercal} \rmS_{i} \in \R^{d_v} \\
&\text{(rest is the same as the attention form)}  \nonumber
\end{align}
where $\rmS$ is the 2-D hidden states of the linear recurrence.

\subsection[RetNet]{RetNet~\citep{sun2023retentive,qin2022devil}}\label{app:retnet}
Based on linear attention, RetNet~\footnote{TransNormer proposed in \citet{qin2022devil} has almost the same architecture as RetNet. } further incorporates rotary positional embeddings~\citep{su2024roformer} and a fixed decay rate $\lambda$. The resulting token mixer, namely \textit{retention}, has the following form. 
\begin{align}
    & \vq_i, \vk_j = \mW_q\vx_i,\mW_k \vx_j  \in \R^{d_k} \\
    & \tilde{\vq}_i, \tilde{\vk}_j = \textrm{RoPE}(\vq_{1:i}), \textrm{RoPE}(\vk_{1:j}) \in \R^{d_k}  \\
    &\mA_{ij} = \lambda^{i-j} \langle \tilde \vq_i,  \tilde \vk_j \rangle \\
    & \vv_j = \mW_v \vx_j \in \R^{d_v}  \\
    & \vz_i = \textrm{retention}(\vx_{1:i}) = \sum_{j=1}^i \mA_{ij} \vv_j \in \R^{d_v} \label{eq:self-att-retnet} \\
    & \vr_i = \mW_r\vx_i \in \R^{d_v} \\
    & \vy_{i} = \mW_o \big( \swish(\vr_i) \odot \vz_{i} \big) \in \R^{d}
\end{align}
While the addition of rotary positional embedding to query/key vectors is straightforward in this attention-style form, the additional decay term $\lambda$ is easier to understand in this equivalent recurrent form.
The linear attention has an equivalent recurrent form as follows.
\begin{align}
& \vq_i, \vk_j = \mW_q\vx_i,\mW_k \vx_j  \in \R^{d_k} \\
& \tilde{\vq}_i, \tilde{\vk}_j = \textrm{RoPE}(\vq_{1:i}), \textrm{RoPE}(\vk_{1:j}) \in \R^{d_k}  \\
& \rmS_{i} = \lambda \rmS_{i-1} +  \tilde \vk_i^\intercal \vv_i \in \R^{d_k \times d_v} \\
&\vz_i = \tilde\vq_i^\intercal \rmS_{i} \in \R^{d_v} \\
 & \text{(rest is the same as the attention form)} \nonumber
\end{align}

\subsection[LSTM]{LSTM~\citep{hochreiter1997long}}\label{app:lstm}
All the recurrences we presented are linear in that the there are no non-linear dependencies between adjacent hidden states, e.g., $\partial \rmS_i / \partial \rmS_{i-1}$ is not a function of $\rmS_{i-1}$. For completeness of recurrences, we also consider LSTM \citep{hochreiter1997long}, which is widely used in the pre-Transformer era.  LSTM uses the following non-linear recurrence,
\begin{align}
   \vf_i &= \sigma (\rmW_f \vx_i + \rmU_f \vh_{i-1}  ) \in \R^{d} \\
   \vi_i &= \sigma (\rmW_i \vx_i + \rmU_i \vh_{i-1} )  \in \R^{d} \\
   \vo_i &= \sigma (\rmW_o \vx_i + \rmU_o \vh_{i-1} )  \in \R^{d} \\
   \tilde \vc_i &= \tanh(\rmW_c \vx_i + \rmU_c \vh_{i-1} ) \in \R^{d} \\
   \vc_i & = \vf_i \odot \vc_{i-1} + \vi_i \odot \tilde \vc_i \in \R^{d}  \\
   \vy_i &= \vo_i \odot \tanh(\vc_i) \in \R^{d} 
\end{align}
where $\vf, \vi, \vo$ denotes forget, input and output gate, respectively. To strictly follow the architecture of traditional multi-layer LSTM, we do not use the feed-forward in-between LSTM layers, i.e., the input of  layer $l$ is directly the output from layer $l-1$.
\subsection[GLA]{GLA~\citep{yang2023gated}}\label{app:gla}

Compared with RetNet, GLA incorporated more fine-grained data-dependent gating. Instead of  using the rotary positional embedding, the fine-grained gates can implicitly capture positional information. For the ease of understanding, we first show the recurrent form of GLA, and then its attention-style form.

For each token, GLA additionally relies on two data dependent decay vectors $\balpha_i \in \R^{d_k}$ and $\bbeta_i \in \R^{d_v}$. The outer-product of them (i.e., $\balpha_i^\intercal \bbeta_i $) decides how much information to preserve from previous hidden state $\rmS_{i-1}$.
\begin{align}
& \vq_i, \vk_j  = \mW_q\vx_i, \mW_k \vx_j  \in \R^{d_k} \\
& \balpha_i = \sigma(\mW_\alpha  \vx_i) \in \R^{d_k} \quad \bbeta_j = \sigma(\mW_\bbeta\vx_j) \in \R^{d_v} \\
& \vv_i = \mW_v \vx_i \in \R^{d_v} \\
& \rmS_{i} = \balpha_i^\intercal \bbeta_i \odot \rmS_{i-1} +  \vk_i^\intercal \vv_i \in \R^{d_k \times d_v} \\
& \vz_i = \vq_i^\intercal \rmS_{i} \in \R^{d_v} \\
& \vr_i = \mW_r\vx_i \in \R^{d_v}   \\
& \vy_{i} = \mW_o \big( \swish(\vr_i) \odot \vz_{i} \big) \in \R^{d}
\end{align}
Like linear attention and RetNet, GLA also has the following attention-style form.~\footnote{Please refer to the original paper for the derivation.}  
\begin{align}
    & \vq_i, \vk_j  = \mW_q\vx_i, \mW_k \vx_j  \in \R^{d_k} \\
    & \balpha_i = \sigma(\mW_\alpha  \vx_i) \in \R^{d_k} \quad \bbeta_j = \sigma(\mW_\bbeta\vx_j) \in \R^{d_v} \\
    & \va_i = \prod_i\balpha_{1:i} \in \R^{d_k} \quad \vb_j = \prod_j\bbeta_{1:j} \in \R^{d_v} \\
    & \vv_j = \mW_v \vx_j \in \R^{d_v} \\
    & \tilde \vq_i = \vq_i \odot \va_i  \in \R^{d_k}  \quad \tilde \vk_j = \vk_j / \va_j \in \R^{d_k}  \quad \tilde \vv_j = \vv_j \odot \vb_j \in \R^{d_v}  \\
    & \vz_{i} = \textrm{gla}(\vx_{1:i}) = \big( \sum_{j=1}^i \mA_{ij} \vv_j\big) / \vb_i   \in \R^{d_v} \\
    & \text{(rest is the same as the recurrent form)}  \nonumber
\end{align}

$\odot$ and $/$ denotes element-wise multiplication and division; $\sigma$ denotes a sigmoid function.

\paragraph{Connections among Linear Attention, RetNet, GLA} 
RetNet and GLA both inherit the basic linear recurrence with 2-D hidden states from linear attention. GLA and RetNet mainly differ in the decaying term from the perspective of the recurrent form. Specifically, GLA incorporates fine-grained data-dependent gates ($\balpha, \bbeta$) whereas RetNet uses a single fixed decay $\lambda$ that is shared across all tokens and hidden dimensions. The simplicity of decay in RetNet leads to neat attention-style form needed for parallel training. In comparison, GLA's attention-style form is more nuanced, thus resulting in a more complex training schema. Moreover, RetNet and GLA incorporate the additional output gate $\vr_i$ before the output projection $\mW_o$. Such output gating is also used in LSTM and RWKV models presented below.

\subsection[RWKV]{RWKV~\citep{peng2023rwkv}}\label{app:rwkv}
The recurrence of RWKV is motivated by attention-free network \citep{zhai2021attention}, and it uses 1-D hidden state compared with the recurrences of linear attention.  
\begin{align}
    &  \vk_i = \mW_k \vx_i \in \R^{d_v} \quad \vv_i = \mW_v \vx_i  \in \R^{d_v} \\
    & \va_i = \exp(-\vw) \odot \va_{i- 1} + \exp(\vk_i) \odot \vv_i \in \R^{d_v} \\
    & \vb_i = \exp(-\vw) \odot \vb_{i - 1} +  \exp(\vk_i)  \in \R^{d_v} \\
    & \vz_i = \textrm{wkv}(\vx_{1:i}) = \frac{\va_{i-1} + \exp(\vk_i + \vu)\odot \vv_i}{\vb_{i-1} + \exp(\vk_i + \vu)}  \in \R^{d_v} \\
    & \vr_i =  \mW_r\vx_i \in \R^{d_v}  \\
    & \vy_{i} = \mW_o \big( \sigma(\vr_i) \odot \vz_i ) \in \R^{d_v} 
\end{align}
where $\vw, \vu \in \R^{d_v}$ are learnable parameters, $\sigma$ is an activation function. The $\textrm{WKV}$ operators maintain a recurrence with a pair of states ($\va_i, \vb_i$). Different from linear attention where the 2D hidden state is constructed via an outer-product $\vk_i^{\intercal} \vv_i$, $\textrm{WKV}$ uses element-wise dot-product $\exp(\vk_i) \odot \vv_i$, thus the shape of the key and value vectors are the same.

Since the decay term $\vw$ is not data-dependent, $\textrm{WKV}$ also has the following equivalent convolutional form:
\begin{align}
    & \vk_i = \mW_k \vx_i \in \R^{d_v} \quad \vv_i = \mW_v \vx_i  \in \R^{d_v} \\
    & \tilde{\vkv}_i =  \exp(\vk_i) \odot \vv_i \in \R^{d_v}  \quad \tilde \vk_i =  \exp(\vk_i) \in \R^{d_v}  \\
    & \vl_i = \exp(-i\vw)   \in \R^{d_v}  \\
     & \va = \vl \ast \tilde{\vkv} \in \R^{L \times d_v}  \\
     & \vb = \vl \ast \tilde \vk \in \R^{L \times d_v} \\
     & \text{(rest is the same as the recurrent form)}   \nonumber
\end{align}
where $\ast$ denotes batched long convolution operator, i.e., one dimension of the filter $\vh[:, i] \in \R^{L \times 1}$ handles one corresponding dimension $\va[:, i], \vb[:, i] \in \R^{L \times 1}$.
 
\subsection[S4]{S4~\citep{gu2021efficiently}}\label{app:s4}

Structured state space models (S4) is a family of sequence models defined with four parameters $(\Delta, \rmA, \rmB, \rmC)$. S4 is typically represented as a sequence mapping of $\R^{L \times 1} \rightarrow \R^{L \times 1}$, wherein the input and output are both scalars (i.e. $\vx, \vy \in \R^{1}$). In this case, S4 has the following recurrent form.
\begin{align}
&\vh_i = \bar \rmA \vh_{i-1} + \bar \rmB \vx_i \in \R^{d_k} \\ 
&\vy_i = \rmC \vh_i \in \R^{1} 
\end{align}
where $d_{\textrm{inner}}$ denotes the dimension of hidden states $\vh_i$, $\bar \rmA \in \R^{d_{\textrm{inner}} \times d_{\textrm{inner}}}$ and $\bar \rmB \in \R^{d_{\textrm{inner}} \times 1}$ are transformed parameters for discrete sequence data according to a certain discretization rule (e.g., zero-order hold). $\rmC \in \R^{1 \times d_{\textrm{inner}}}$. Equivalently, it has the following convolutional form:
\begin{align}
&\bar \rmK = [\rmC\bar\rmB, \rmC\bar\rmA\bar\rmB, \dots \rmC\bar\rmA^{L-1}\bar\rmB] \\    
&\vy = \vx \ast \bar \rmK
\end{align}
where $\ast$ denotes the convolution operator and $\bar \rmK $ denotes the convolution kernel. The convolution form is critical on enabling efficient parallel training via Fast Fourier Transform (FFT) algorithms.

Since the recurrent forms of other models are usually presented with vector input/output (i.e., $\vx_i, \vy_i \in \R^{d}$), we present its equivalent batched recurrent form as follows:
\begin{align}
    &\rmS_i = \bar \rmA \circ \rmS_{i-1} + \bar \rmB \circ \vx_i \in \R^{d \ \times d_{\textrm{inner}}} \\
    &\vy_i = \rmC \circ \rmS_i  \in \R^{d} \label{eq:s4-batched}
\end{align}
where $\rmS_i$ denotes 2-D hidden states, $\rmA \in \R^{d  \times d_{\textrm{inner}} \times  d_{\textrm{inner}}}, \rmB \in \R^{d \times  d_{\textrm{inner}} \times 1}, \rmC \in \R^{d \times 1 \times d_{\textrm{inner}}}$, $\circ$ denotes batched matrix multiplication.~\footnote{To differentiate the size of hidden states. in recurrences, we use $\vh_i$ in the 1-D cases; $\rmS_i$ in the 2-D cases.} In this batched form, $d$ numbers of independent SSM run in parallel, each responsible for a dimension of input $\vx$.

\paragraph{Connections to Linear Attentions}
With this batched form in \cref{eq:s4-batched}, it becomes clear that S4, similar to linear attention, enjoys a large 2-D hidden states for recurrence. We can also draw a rough parallel between ($\bar \rmB$, $\rmC$) in S4 to ($\vq_i, \vk_j$) in linear attention as they handle the input and output for the recurrences, respectively. The parallel reveals the difference between S4 and linear attention. In S4, the input and output mapping is not data-dependent, i.e., ($\bar \rmB$, $\rmC$) does not depend on input $\vx$. In comparison, $\vq_i$ and $\vk_j$ are linear mappings of the input $\vx_i$. 

\subsection[H3]{H3~\citep{dao2022hungry}} \label{app:h3}
H3 is a mixture of state-space models and linear attention. In particular, it employs the outer-product structure from linear attention (i.e., $\vk_i^T \vv_i$) to construct the input of a state-space model. 
\begin{align}
    & \vk_i = \mW_k \vx_i \in \R^{d_k} \quad \vv_i =  \mW_v\vx_i \in \R^{d_v} \\
    & \vx'_i = \vk_i^\intercal \vv_i \in \R^{d_k \times d_v} \\
    &  \rmS_i = \bar \rmA  \odot \rmS_{i-1} + \bar \rmB \odot\vx'_i  \in \R^{d_k \times d_v \times d_{\text{inner}}} \qquad   \\
    & \vz'_i =  \rmC \circ \rmS_i    \in \R^{d_k \times d_v} \\
    & \vq_i = \mW_q\vx_i  \in \R^{d_k} \\
    & \vz_i = \vq_i \vz'_i \in \R^{d_v} \\
    & \vy_i = \vz'_i \mW_o \in \R^{d} 
\end{align}
where $\bar \rmA$, $\bar \rmB$, $\rmC \in \R^{d_{\textrm{inner}}}$ are parameters of the state-space models, $\odot$ denotes element-wise product with broadcasting, $\circ$ denotes batched matrix-vector product. The SSM is diagonally parameterized (i.e., $\bar \rmA$ is a vector) and the original H3 paper additionally uses another shift-SSM \citep{dao2022hungry} to further refine the key vector $\vk_i$.

\subsection[Hyena]{Hyena~\citep{poli2023hyena}}\label{app:hyena}

Hyena is a pure convolutional model that does not have an equivalent recurrent form, unlike S4. 
However, it recursively applies the convolution operator at the sequence level for $N$ times (i.e., order-$N$ Hyena). In practice, $N$ is usually set to be $2$, and the resulting form is as follows. 

\begin{align}
  & \vv^n = \mW_{n}\vx \in \R^{L \times d} \\
  & \vz^{0}=  \vv^0 \in \R^{L \times d} \\
  & \begin{rcases}
       & \vl^n_i = \operatorname{FFN}(\vi) \in \R^{L \times d} \\
       & \vz^n = \vv^{n-1} \odot (\vl^n  \ast \vz^{n-1}) \in \R^{L \times d} 
  \end{rcases} \text{ recursion } n=1 \dots N \label{eq:hyena-conv} \\
  & \vy = \vz^N \in \R^{L \times d}
\end{align}

where $\ast$ denotes batched convolution operator. In practice, the filter is padded to the size of $(2L - 1) \times d$ so that the convolution operator becomes a circular convolution for efficient training using FFT.~\footnote{Please refer to Section 2 and 3 of \citep{poli2023hyena} for details.}
Note that the resulting kernels $\vl^1, \vl^2$ do not depend on input $\vx$, but the convolution output is controlled by the data-dependent gate $\vv^1, \vv^2$ in \cref{eq:hyena-conv}. %

\subsection[Mamba]{Mamba~\citep{gu2023mamba}}\label{app:mamba}
Mamba has the same recurrent form as S4, and uses data-dependent parameterization for $\bar \rmA$, $\bar \rmB$, $\rmC$:
\begin{align}
    & \vv_i = \mW_v \vx_i  \in \R^{d_v} \\
    & \rmS_i = \bar \rmA_i \odot \rmS_{i-1} + \bar \rmB_i \odot \vv_i \in \R^{d_k \times d_v} \quad (\text{$\odot$ with broadcast}) \\
    & \vy_i =  \rmC_i  \rmS_i \in \R^{d_v} 
\end{align}
where $\bar \rmA_i, \bar \rmB_i \in \R^{d_k \times d_v}$, $\rmC_i \in \R^{d_v}$ data-dependently parameterized, i.e., computed based on $\vx_i/\vv_i$. However, due to the data-dependence, this recurrent form no longer has an equivalent convolutional form for efficient training. The original paper handles this issue with customized hardware-efficient training algorithms based on the recurrent form.

\section{Optimization \& Hyperparameter Search}
\begin{table}[ht]
    \centering
    \begin{tabular}{ll}
        \toprule
         \bf Hyper Parameter  & \bf Search \\ \midrule
         hidden size & [64, 128, 256, 512, 1024] \\
         number of layers & [1, 2, 4, 8, 12]\\
         number of heads & [1, 2, 4] \\
         epochs & [200, 400]  \\
         batch size & 32 \\
         optimizer & [AdamW] \\
         \boxSpace\boxRight learning rate & [1e-4, 2.5e-4 ] \\
         \boxSpace\boxRight  weight decay & [0.01, 0.1] \\
         \boxSpace\boxRight $\beta$s &  [(0.9, 0.99)] \\
         scheduler & Cosine Scheduler with Warmup \\
          \boxSpace\boxRight minimum learning rate & 2.5e-5 \\
          \boxSpace\boxRight warm-up start learning rate & 1e-7 \\
          \boxSpace\boxRight warm-up steps & 25000 \\
         \bottomrule
    \end{tabular}
    \caption{Hyper-parameter search space for neural models.}
    \label{tab:hyperparam}
\end{table}
We brute force search over grid of hyper-parameters in \cref{tab:hyperparam} and pick the best setting best on validation set on ICLL and AR seperately. In AR we searched hidden sizes up to 256. In ICLL, we search first upto hidden size of 256, then if the best performing hidden size is 256, we try 512, and then 1024. We also used only best performing weight decay of 0.1 and learning rate of 2.5e-4 in the additional search runs. 

\section{Algorithms}\label{app:algs}
\subsection{In-context N-gram Language Model}\label{app:n-gram}
\begin{figure}[ht]
\centering
\begin{minipage}{0.6\linewidth}
\input{algos/ngram}
\end{minipage}
\end{figure}

In \cref{alg:ngram}, we present an \textbf{in-context} applied n-gram model that incorporates a back-off mechanism \citep{chen1999empirical}. This model differs from the standard n-gram approach that is trained on the training set. Instead, here we train a unique n-gram for each example at each time step to predict the subsequent word. The back-off strategy allows for the assignment of non-zero probabilities to unseen n-grams by utilizing information from lower-order n-grams, as shown in line 14 of \cref{alg:ngram}. For each n-gram context $x_{i-N+1}^{i-1}$, the back-off weight $\beta(x_{i-N+1}^{i-1})$ can be computed as follows:

\begin{equation}
    \beta(x_{i-N+1}^{i-1}) = 1 - \sum_{\{w \mid c(x_{i-N+1}^{i-1}w) > 0\}}  \frac{c^{*}(x_{i-N+1}^{i-1}w)}{c^{*}(x_{i-N+1}^{i-1})}
\end{equation}

In the absence of smoothing, the summation is expected to equal 1, resulting in $\beta$ being 0. Smoothing techniques, such as laplace smoothing, modify the counts and allocate a probability mass for unseen n-grams. Alternatively, by excluding the probability corresponding to the padding token $w$, we can reserve probability mass for back-off without explicit smoothing. This approach is employed in our n-gram model implementation and it worked slightly better than add-one smoothing.

Finally, the back-off weights $\alpha$ calculated by normalizing beta for the lower-order n-gram probabilities for the unseen current n-gram sequences:

\begin{equation}
    \alpha(x_{i-N+1}^{i-1}) = \frac{\beta(x_{i-N+1}^{i-1})}{\mathop{\sum}_{\{w \mid c(x_{i-N+1}^{i-1}w) = 0\}}  P(w \mid x_{i-N+2}^{i-1})}
\end{equation}

It is important to note that the normalization ensures that the probabilities of all potential continuations of a given context sum to one.

\subsection{In-context Baum-Welch HMM Language Model}\label{app:bw}
\begin{figure}[ht]
\centering
\begin{minipage}{0.8\linewidth}
\input{algos/bw}
\end{minipage}
\end{figure}
Given a probabilistic automaton, \texttt{PFA}, from \ourdataset, we can construct a Hidden Markov Model (HMM) that assigns the same probabilities to any given string. The construction can be done as:
\begin{itemize}
    \item For each pair of states $S_i, S_j \in \mathcal{S}$, create a corresponding HMM state $H_{(S_i, S_j)}$.
    \item Define the transition probabilities $A(H_{(S_i, S_j)}, H_{(S_l, S_m)}) \propto 1[j=l] \cdot T_{\texttt{PFA}}(S_i, w, S_j)$, where each character $w$ transitions to a unique state in our \texttt{PFA}s.
    \item Set the emission probabilities $B({H_{(S_i, S_j)}, w}) = 1$ if $T_{\texttt{PFA}}(S_i, w, S_j) > 0$, and $0$ otherwise.
    \item Set initial state probabilities 1 for the start states and 0 for the others: $\pi( H_{(S_i, S_j)}) = 1[i==1]$
    
\end{itemize}

The number of states in the constructed HMM is the square of the number of states in the probabilistic automaton. Therefore, we fit an HMM to the examples in \ourdataset with a maximum of $\textrm{NS} = 12^2 = 144$ states. Algorithm \cref{alg:bw} details the in-context Baum-Welch predictor. We begin by constructing a list of observations from the current prefix $x_{1:{i-1}}$, and then fit an HMM given the global vocabulary $\mathcal{V}$ and number of states $\textrm{NS} = 144$ using an improved Baum-Welch algorithm that is consistent with the structure of probabilistic automata in \ourdataset. We incorporate two pieces of prior information about the dataset:

\subsection[Masking A to enforce state transitions]{Masking $A$ to enforce state transitions}\label{app:mask_A}
In our construction, we assume $A_{H_{(S_i, S_j)}H_{(S_l, S_m)}} = 0$ if $j \neq l$. We enforce this constraint in each iteration by masking the corresponding entries in $A$. Additionally, as our PFA sampling schema in \cref{sec:samp-lang} does not include self-transitions, we set all $A_{H_{(S_i, S_i)}H_{(S_i, S_l)}} = 0$.

\subsection[Masking pi to start at the initial states]{Masking $\pi$ to start at the initial state}\label{app:mask_pi}
All our PFAs have a single start state, which we denote as $H_{(S_0, S_i)}$ for all $i$, without loss of generality. We mask all other initial state probabilities such that $\pi(H_{(S_0, S_i)}) = 0$ for $i \neq 0$.

In our experiments, these masking strategies significantly improved the accuracy of the Baum-Welch algorithm. The results presented are based on this modified BW algorithm.

\section{Learned MLP Reweighting}\label{app:mlpsm}
We provide the training details of MLP n-gram reweighting models' used in \cref{sec:whichalgo}, namely LNW, LNW$_r$, and LNW$_b$. 

\paragraph{Count Features (LNW Model)}
Given a data point $d = x_0 \dots x_i \dots x_l = x_0^{l}$, we first extract n-gram features for each position $i$ and for each n-gram length $n$:
\begin{equation}
\textrm{gram}(i; n) = \left[ \textrm{count}_{x_{1:i}}(x_{i-n}^{i-1} w) - 1 \quad \forall w \in \mathcal{V} \right] \in \mathcal{Z}^{|\mathcal{V}|} 
\end{equation}
The full set of n-gram features is the concatenation of n-gram features for $n=1$ to $n=3$:
\begin{equation}
    \textrm{gram}(i; \leq3) = \textrm{concatenate}(\textrm{gram}(i; 1), \textrm{gram}(i; 2), \textrm{gram}(i; 3)) \in \mathcal{Z}^{3|\mathcal{V}|} 
\end{equation}

We then train a sequence model that takes $\textrm{gram}(i; \leq 3)$ as input and applies a 2-layer MLP with GeLU activation to produce the unnormalized scores for the next token distribution. We use the same language modeling loss as in \cref{eq:lm}. Our hyper-parameters for MLP training are as follows:
\begin{center}
\begin{tabular}{ll}
    \toprule
    \textbf{hyper parameter} & \textbf{value} \\ \midrule
    hidden size & 1024 \\
    epochs & 50 \\
    batch size & 32  \\
    optimizer & Adam \\
    \boxSpace\boxRight learning rate & 1e-3\\
    \boxSpace\boxRight $\beta$s & (0.9, 0.99) \\
    scheduler & reduce on plateu \\
    \boxSpace\boxRight patiance & 5 epochs \\
    \boxSpace\boxRight factor & 0.5 \\ 
    \boxSpace\boxRight minimum learning rate  & 1e-5\\
    \bottomrule
\end{tabular}
\end{center}

\paragraph{Frequency Features (LNW$_r$ Model)}
The frequency features model uses normalized n-gram features $\frac{\textrm{gram}(i; n)}{\sum \textrm{n-gram}(i; n)}$ instead of the raw n-gram features explained above.

\paragraph{Binary Features (LNW$_b$ Model)}
The binary features model uses n-gram existence features, where $\textrm{n-gram}(i; n) = 1$ if the n-gram exists at position $i$ and $0$ otherwise, instead of raw n-gram features.

\section{Probing Experiments}\label{app:probing}
\begin{figure}
    \centering
    \includegraphics[width=\textwidth]{figures/probes_40k.pdf}
    \caption{Additional results on probing analysis of n-gram representations with neural sequence models trained with $N_{\textrm{train}}=40000$ examples. See \cref{fig:prob25} for details.}
    \label{fig:probe400}
    \vspace{-6mm}
\end{figure}

\paragraph{Model and Objective}
We train a 2-layer Multilayer Perceptron (MLP) as our probe model in two configurations: \textbf{(1)} $f_{\textrm{n-gram}}(\vh, \vc)$, where $\vh$ represents a hidden state at a specific time step and $\vc$ denotes the query n-gram; and \textbf{(2)} $f_{\textrm{equal}}(\vh_i, \vh_j)$, which is employed in state equivalence probes. The formulation of our $f_{\textrm{n-gram}}(\vh, \vc)$ for an n-gram probe is as follows:
\begin{align}
    \ve_c &=  \mW_{\textrm{embed}}\vc \in \mathbb{R}^{n \times d/2} \\
    \ve_c &= \operatorname{flatten}(\ve_c) \in \mathbb{R}^{nd/2} \\
    \ve_h  &= \mW_{\textrm{proj}}\vh \in \mathbb{R}^{nd/2} \\
    \vx &=\operatorname{concatenate}([\ve_c, \ve_h, \ve_c \odot \ve_h])\\
    \vy &= \mW_2 \operatorname{GeLU}(\mW_1 \vx + \vb_1) + \vb_2
\end{align}
where $n$ is the order of the n-gram and $d$ is the dimensionality of the hidden state used by the probe.
For regression tasks, we employ the mean squared error loss on the output and our targets are corresponding n-gram counts or frequencies. While for classification tasks, we utilize binary cross-entropy loss with the logits being $\vy$, and targets are whether the corresponding n-gram exists or not. 
\paragraph{Data}
We train the probe using hidden states extracted from the actual training set of the models. Specifically, we randomly select an example from the training set, randomly choose a time step within that example, and then create a query n-gram by appending a random next character to the last $n-1$ characters at the chosen time step. For regression tasks, we only consider n-grams that appear at least once in the prefix. Each epoch involves iterating over each example once. For testing, we apply the same sampling procedure using hidden states from the test set.
\paragraph{Model and Objective}
The state equivalence probe $f_{\textrm{equal}}(\vh_i, \vh_j)$ is defined as:
\begin{align}
    \ve_{i}  &= \mW_{\textrm{proj}}\vh_i \in \mathbb{R}^{d} \\
    \ve_{j}  &= \mW_{\textrm{proj}}\vh_j \in \mathbb{R}^{d} \\
    \vx &=\operatorname{concatenate}([\ve_i, \ve_j, \ve_i \odot \ve_j]) \in \mathbb{R}^{3d}\\
    \vy &= \mW_2 \operatorname{GeLU}(\mW_1 \vx + \vb_1) + \vb_2
\end{align}
where $d$ is the dimensionality of the hidden state used by the probe. 
We use the cross-entropy loss in the classification of whether two states are equivalent, and 
$\vy$ serves as the logits for cross-entropy.
\paragraph{Data}
Similar to the n-gram probe, we train the state equivalence probe using hidden states from the model's training set. We randomly select an example and then sample two time steps within it, ensuring that in 50\% of cases the probe receives identical states, and in the remaining 50\%, it receives different states. The testing procedure mirrors that of the training phase.

We employ the following hyperparameters for all probe training. 
We train separate probes for each layer and present the best results in \cref{fig:prob25} and \cref{fig:probe400}.
\begin{center}
\begin{tabular}{ll}
    \toprule
    \textbf{hyper parameter} & \textbf{value} \\ \midrule
    hidden size ($d$) & 128 \\
    epochs & 1000 \\
    batch size & 64  \\
    optimizer & Adam \\
    \boxSpace\boxRight learning rate & 3e-4\\
    \boxSpace\boxRight $\beta$s & (0.9, 0.99) \\
    scheduler & Cosine Annealing  \\
    \boxSpace\boxRight minimum learning rate  & 1e-4\\
    \bottomrule
\end{tabular}
\end{center}

\section{Implementations of N-gram Layers}
In \cref{fig:ngramheadcode} and \cref{fig:ngrammodulecode}, we provide a Python implementation for n-gram layers that we use in our experiments.
\begin{figure}[H]
\begin{python}
def ngram_head(x, hidden_state, shift_step=1, ngram=1):
    """
    Args:
        x: bsz * input_len
        hidden_state: bsz * input_len * d_model
        ngram: 1 means bigram, 2 means trigram
        shift_step: which token to attend to after the matching ngram
    Output:
        bsz * input_len * d_model
    """
    bsz, seq_len = x.shape
    # bsz * L * L, match unigram as the first step
    mask_0 = x[:, None, :] == x[:, :, None]
    causal_mask = torch.tril(torch.ones(seq_len, seq_len, 
        dtype=torch.bool, device=x.device), diagonal=-1 )
    mask_0 = torch.logical_and(mask_0, causal_mask)

    masks = [mask_0.long()]
    for _ in range(1, ngram):
        # mask_0[i, j] = True means token i-1 and token j-1 is matched
        mask_0 = F.pad(mask_0, (1, -1, 1, -1), "constant", False)
        masks.append(mask_0.long())
    ngram_mask = torch.stack(masks, dim=-1).sum(dim=-1) >= ngram
    if shift_step > 0:
        ngram_mask = F.pad(ngram_mask, 
            (shift_step, -shift_step), "constant", False)
    ngram_mask = torch.logical_and(ngram_mask, causal_mask)

    # form a uniform distribution for matched tokens
    ngram_mask_norm = ngram_mask / ngram_mask.sum(dim=2, keepdim=True)
    ngram_mask_norm = torch.nan_to_num(ngram_mask_norm, 0)
    ngram_mask_norm = ngram_mask_norm.to(hidden_state.dtype) 
    output = torch.einsum("bmn,bnz->bmz", ngram_mask_norm, hidden_state)
    return output

class Ngram(nn.Module):
    def __init__(self, d_model, ngram=1):
        super().__init__()
        self.d_model = d_model
        self.ngram = ngram
        self.t0 = nn.Linear(self.d_model, self.d_model)
        self.t1 = nn.Linear(self.d_model, self.d_model)

    def forward(self, x, input_ids):
        bsz, seq_len, _ = x.shape
        h0 = ngram_head(input_ids, x, ngram=self.ngram)
        h1 = x
        y = self.t0(h0) + self.t1(h1)
        return y
\end{python}
\caption{Python implementation of n-gram layers.}
\label{fig:ngramheadcode}
\end{figure}

\begin{figure}[H]
\begin{python}
class NgramBlock(nn.Module):
    def __init__(self, config, ngram):
        """
        Args:
            ngram: 1, 2, or 3
            
        Note: parameter size 4d^2
        """
        super().__init__()
        self.ln_1 = RMSNorm(config.d_model, eps=1e-5)
        
        self.attn = Ngram(config, ngram)
        self.ln_2 = RMSNorm(config.d_model, eps=1e-5)

        mlp_hidden = config.d_model 
        self.mlp = nn.Sequential(
            nn.Linear(config.d_model, mlp_hidden),
            nn.SiLU(),
            nn.Linear(mlp_hidden, config.d_model),
        )

    def forward(self, x, input_ids):
        x_att = self.attn(self.ln_1(x), input_ids)
        x = x + x_att
        x_mlp = self.mlp(self.ln_2(x))
        x = x + x_mlp
        return x
 
\end{python}
\caption{Python implementation of n-gram blocks with SwiGLU-MLP~\citep{shazeer2020glu} and RMSNorm~\citep{zhang2019root}.}
\label{fig:ngrammodulecode}
\end{figure}

\section{Language Model Experiments}
In the language model experiments, all models share the same following training hyperparameters. 
We plan to extend the experiment setting to larger models trained with more tokens in the future.

\begin{center}
\begin{tabular}{ll}
    \toprule
    \textbf{hyper parameter} & \textbf{value} \\ \midrule
    hidden size ($d$) & 1024 \\
    number of training tokens & 7e9 \\
    number of warm-up tokens & 5e8 \\
    batch size (number of tokens) & 5e5   \\
    optimizer & AdamW \\
    weight decay & 0.01 \\
    \boxSpace\boxRight learning rate & 3e-4\\
    \boxSpace\boxRight $\beta$s & (0.9, 0.95) \\
    scheduler & Cosine Annealing  \\
    \boxSpace\boxRight minimum learning rate  & 3e-5\\
    \bottomrule
\end{tabular}
\end{center}
