# Supplementary material for: Learning Syntax Without Planting Trees: Understanding Hierarchical Generalization in Transformers
Source: arXiv:2404.16367 source file (2025-03-16)
Supplement: Supplementary file 2 [file hybrid_models.tex]

\captionsetup{position=top}

\begin{table}
\centering
\subfloat[{\textbf{n-gram layers bring other models to the Transormer level on ICLL}: We train RetNet and GLA models with n-gram heads on ICLL with $N=2500$ training examples. In TVD metric, adding n-gram layers, brings model performance to the Transformer level trained on the same data without n-gram heads.. In accuracy, hybrid models can outperform Transformer models in the accuracy metric.}]{  
\resizebox{.45\textwidth}{!}{
\begin{tabular}{lll}
\toprule
\multicolumn{1}{c}{\textbf{Model}}  & \multicolumn{1}{c}{\textbf{TVD ($\downarrow$)}} & \multicolumn{1}{c}{\textbf{Accuracy ($\uparrow$)}}\\
\midrule
RetNet \citep{sun2023retentive} & 0.392 & 0.800\\
 \boxSpace\boxRight  \texttt{NGH}$_1^{(1)}$ & 0.310 & 0.814 \\
  \boxSpace\boxRight  \texttt{NGH}$_1^{(1,2)}$ & 0.229 & 0.925 \\
   \boxSpace\boxRight  \texttt{NGH}$_1^{(1,2,3)}$ & 0.217 & 0.94\\
 \midrule
GLA \citep{yang2023gated} & 0.624 & 0.526  \\
 \boxSpace\boxRight  \texttt{NGH}$_1^{(1)}$ & 0.302 & 0.819 \\ 
 \boxSpace\boxRight  \texttt{NGH}$_1^{(1,2)}$ & 0.211 & 0.929 \\ 
 \boxSpace\boxRight  \texttt{NGH}$_1^{(1,2,3)}$ & 0.207 & \textbf{0.946} \\ \midrule
 Transformer \citep{vaswani2017attention} & \textbf{0.203} & 0.926 \\
\bottomrule
\end{tabular}
}} \hfill \subfloat[{\textbf{n-gram layers improves language models}: We train equal sized (340M parameters) language models with and without n-gram heads on 7B tokens from the SlimPajama dataset \citep{cerebras2023slimpajama}. Adding n-gram layers improves each models performance regardless of the model by reducing test set perplexities up to 1.14 point.}]{
\resizebox{.45\textwidth}{!}{
\begin{tabular}{ll}
\toprule
\multicolumn{1}{c}{\textbf{Model}}  & \multicolumn{1}{c}{\textbf{Perplexity ($\downarrow$)}} \\ \midrule
RetNet  \citep{sun2023retentive}           & 16.55        \\
 \boxSpace\boxRight  \texttt{NGH}$_1^{(1,2,3)}$ +  \texttt{NGH}$_{-2}^{(1,2,3)}$  & 15.86 (\textbf{+4.2\%})           \\\midrule
GLA \citep{yang2023gated}                & 15.65    \\
 \boxSpace\boxRight   \texttt{NGH}$_1^{(1,1,1)}$ + \texttt{NGH}$_{-2}^{(1,1,1)}$     & 15.54  (\textbf{+0.7\%})   \\ 
 \boxSpace\boxRight  \texttt{NGH}$_1^{(1,2,3)}$ +  \texttt{NGH}$_{-2}^{(1,2,3)}$     & 15.24  (\textbf{+2.6\%})     \\ \midrule
 Transformer (Llama) \citep{touvron2023llama}      & 16.96         \\
\boxSpace\boxRight \texttt{NGH}$_1^{(1,2,3)}$+  \texttt{NGH}$_{-2}^{(1,2,3)}$    & \textbf{15.82} (\textbf{+6.7\%})        \\
\bottomrule
\end{tabular}
}}
\captionof{table}{\textbf{Hybrid model experiments on ICLL and language modeling.}}
\label{tbl:hybridmodels}%
\end{table}
