# Supplementary material for: Learning Syntax Without Planting Trees: Understanding Hierarchical Generalization in Transformers
Source: arXiv:2404.16367 source file (2025-03-16)
Supplement: Supplementary file 3 [file hyperparameter.tex]

\begin{table}[ht]
    \centering
    \begin{tabular}{ll}
        \toprule
         \bf Hyper Parameter  & \bf Search \\ \midrule
         hidden size & [64, 128, 256, 512, 1024] \\
         number of layers & [1, 2, 4, 8, 12]\\
         number of heads & [1, 2, 4] \\
         epochs & [200, 400]  \\
         batch size & 32 \\
         optimizer & [AdamW] \\
         \boxSpace\boxRight learning rate & [1e-4, 2.5e-4 ] \\
         \boxSpace\boxRight  weight decay & [0.01, 0.1] \\
         \boxSpace\boxRight $\beta$s &  [(0.9, 0.99)] \\
         scheduler & Cosine Scheduler with Warmup \\
          \boxSpace\boxRight minimum learning rate & 2.5e-5 \\
          \boxSpace\boxRight warm-up start learning rate & 1e-7 \\
          \boxSpace\boxRight warm-up steps & 25000 \\
         \bottomrule
    \end{tabular}
    \caption{Hyper-parameter search space for neural models.}
    \label{tab:hyperparam}
\end{table}
