# Supplementary material for: Learning Syntax Without Planting Trees: Understanding Hierarchical Generalization in Transformers
Source: arXiv:2404.16367 source file (2025-03-16)
Supplement: Supplementary file 4 [file models.tex]

\subsection[Transformers with Self Attention]{Transformers with Self Attention \citep{vaswani2017attention}}\label{app:transformers}
Standard self-attention performs token mixing in the following way:
\begin{align}
    & \vq_i, \vk_j  = \mW_q\vx_i ,\mW_k \vx_j  \in \R^{d_k}   \\
    & \mA_{ij}  \propto \exp(\langle \vq_i, \vk_j \rangle) \in (0,1) \qquad \text{softmax attention} \\
    & \vv_j = \mW_v \vx_j \in \R^{d_v} \\
    & \vz_{i} = \sum_{j=1}^i \mA_{ij} \vv_j \in \R^{d_v} \label{eq:self-att}  \\
    & \vy_{i} = \mW_o \vz_{i} \in \R^{d}
\end{align}
where $d_k, d_v$ denote the dimension for query/key and value vectors, respectively. 
The attention scores are computed based on the pairwise dot-product between the query vector of the current token and key vectors from the context. In the multi-head attention, attention output $\vz_i$ is independently computed  in each head; all outputs are concatenated as the final attention output, which will then be fed into the output projection $\mW_o$. %

\subsection[Transformers with Linear Attention]{Transformers with Linear Attention~\citep{katharopoulos2020transformers}}\label{app:lineartransformers}

The linear attention~\citep{katharopoulos2020transformers} simplifies the standard attention by replacing $\exp(\langle \vq_i, \vk_j \rangle)$ with a kernel map $k(\vq_i, \vk_j )$ with an associative feature map (i.e., $k(\vq_i, \vk_j ) = \phi(\vq_i) \phi(\vk_j)$). In this work, we consider a simple feature map of identity function (i.e., $\phi(\vq_i) = \vq_i$), which yields surprisingly good performance for language model on real data in recent works~\citep{qin2022devil,yang2023gated}. With this feature map, the token mixing process is very similar to standard attention, except that attention scores are not normalized.%
\begin{align}
& \vq_i, \vk_j =  \mW_q\vx_i ,\mW_k \vx_j  \in \R^{d_k}  \\
& \mA_{ij} = \langle \vq_i, \vk_j \rangle \qquad \text{linear attention}   \\
& \vv_j = \mW_v \vx_j \in \R^{d_v}  \\
& \vz_{i} = \sum_{j=1}^i \mA_{ij} \vv_j \in \R^{d_v} \qquad \label{eq:self-att-linear} \\
&  \vy_{i} = \mW_o \vz_{i} \in \R^{d}
\end{align}

The linear attention has an equivalent recurrent form as follows.
\begin{align}
& \vq_i, \vk_j =  \mW_q\vx_i ,\mW_k \vx_j  \in \R^{d_k}  \\
& \rmS_{i} = \rmS_{i-1} + \vk_i^\intercal \vv_i \in \R^{d_k \times d_v} \\
&\vz_i = \vq_i^{\intercal} \rmS_{i} \in \R^{d_v} \\
&\text{(rest is the same as the attention form)}  \nonumber
\end{align}
where $\rmS$ is the 2-D hidden states of the linear recurrence.

\subsection[RetNet]{RetNet~\citep{sun2023retentive,qin2022devil}}\label{app:retnet}
Based on linear attention, RetNet~\footnote{TransNormer proposed in \citet{qin2022devil} has almost the same architecture as RetNet. } further incorporates rotary positional embeddings~\citep{su2024roformer} and a fixed decay rate $\lambda$. The resulting token mixer, namely \textit{retention}, has the following form. 
\begin{align}
    & \vq_i, \vk_j = \mW_q\vx_i,\mW_k \vx_j  \in \R^{d_k} \\
    & \tilde{\vq}_i, \tilde{\vk}_j = \textrm{RoPE}(\vq_{1:i}), \textrm{RoPE}(\vk_{1:j}) \in \R^{d_k}  \\
    &\mA_{ij} = \lambda^{i-j} \langle \tilde \vq_i,  \tilde \vk_j \rangle \\
    & \vv_j = \mW_v \vx_j \in \R^{d_v}  \\
    & \vz_i = \textrm{retention}(\vx_{1:i}) = \sum_{j=1}^i \mA_{ij} \vv_j \in \R^{d_v} \label{eq:self-att-retnet} \\
    & \vr_i = \mW_r\vx_i \in \R^{d_v} \\
    & \vy_{i} = \mW_o \big( \swish(\vr_i) \odot \vz_{i} \big) \in \R^{d}
\end{align}
While the addition of rotary positional embedding to query/key vectors is straightforward in this attention-style form, the additional decay term $\lambda$ is easier to understand in this equivalent recurrent form.
The linear attention has an equivalent recurrent form as follows.
\begin{align}
& \vq_i, \vk_j = \mW_q\vx_i,\mW_k \vx_j  \in \R^{d_k} \\
& \tilde{\vq}_i, \tilde{\vk}_j = \textrm{RoPE}(\vq_{1:i}), \textrm{RoPE}(\vk_{1:j}) \in \R^{d_k}  \\
& \rmS_{i} = \lambda \rmS_{i-1} +  \tilde \vk_i^\intercal \vv_i \in \R^{d_k \times d_v} \\
&\vz_i = \tilde\vq_i^\intercal \rmS_{i} \in \R^{d_v} \\
 & \text{(rest is the same as the attention form)} \nonumber
\end{align}

\subsection[LSTM]{LSTM~\citep{hochreiter1997long}}\label{app:lstm}
All the recurrences we presented are linear in that the there are no non-linear dependencies between adjacent hidden states, e.g., $\partial \rmS_i / \partial \rmS_{i-1}$ is not a function of $\rmS_{i-1}$. For completeness of recurrences, we also consider LSTM \citep{hochreiter1997long}, which is widely used in the pre-Transformer era.  LSTM uses the following non-linear recurrence,
\begin{align}
   \vf_i &= \sigma (\rmW_f \vx_i + \rmU_f \vh_{i-1}  ) \in \R^{d} \\
   \vi_i &= \sigma (\rmW_i \vx_i + \rmU_i \vh_{i-1} )  \in \R^{d} \\
   \vo_i &= \sigma (\rmW_o \vx_i + \rmU_o \vh_{i-1} )  \in \R^{d} \\
   \tilde \vc_i &= \tanh(\rmW_c \vx_i + \rmU_c \vh_{i-1} ) \in \R^{d} \\
   \vc_i & = \vf_i \odot \vc_{i-1} + \vi_i \odot \tilde \vc_i \in \R^{d}  \\
   \vy_i &= \vo_i \odot \tanh(\vc_i) \in \R^{d} 
\end{align}
where $\vf, \vi, \vo$ denotes forget, input and output gate, respectively. To strictly follow the architecture of traditional multi-layer LSTM, we do not use the feed-forward in-between LSTM layers, i.e., the input of  layer $l$ is directly the output from layer $l-1$.
\subsection[GLA]{GLA~\citep{yang2023gated}}\label{app:gla}

Compared with RetNet, GLA incorporated more fine-grained data-dependent gating. Instead of  using the rotary positional embedding, the fine-grained gates can implicitly capture positional information. For the ease of understanding, we first show the recurrent form of GLA, and then its attention-style form.

For each token, GLA additionally relies on two data dependent decay vectors $\balpha_i \in \R^{d_k}$ and $\bbeta_i \in \R^{d_v}$. The outer-product of them (i.e., $\balpha_i^\intercal \bbeta_i $) decides how much information to preserve from previous hidden state $\rmS_{i-1}$.
\begin{align}
& \vq_i, \vk_j  = \mW_q\vx_i, \mW_k \vx_j  \in \R^{d_k} \\
& \balpha_i = \sigma(\mW_\alpha  \vx_i) \in \R^{d_k} \quad \bbeta_j = \sigma(\mW_\bbeta\vx_j) \in \R^{d_v} \\
& \vv_i = \mW_v \vx_i \in \R^{d_v} \\
& \rmS_{i} = \balpha_i^\intercal \bbeta_i \odot \rmS_{i-1} +  \vk_i^\intercal \vv_i \in \R^{d_k \times d_v} \\
& \vz_i = \vq_i^\intercal \rmS_{i} \in \R^{d_v} \\
& \vr_i = \mW_r\vx_i \in \R^{d_v}   \\
& \vy_{i} = \mW_o \big( \swish(\vr_i) \odot \vz_{i} \big) \in \R^{d}
\end{align}
Like linear attention and RetNet, GLA also has the following attention-style form.~\footnote{Please refer to the original paper for the derivation.}  
\begin{align}
    & \vq_i, \vk_j  = \mW_q\vx_i, \mW_k \vx_j  \in \R^{d_k} \\
    & \balpha_i = \sigma(\mW_\alpha  \vx_i) \in \R^{d_k} \quad \bbeta_j = \sigma(\mW_\bbeta\vx_j) \in \R^{d_v} \\
    & \va_i = \prod_i\balpha_{1:i} \in \R^{d_k} \quad \vb_j = \prod_j\bbeta_{1:j} \in \R^{d_v} \\
    & \vv_j = \mW_v \vx_j \in \R^{d_v} \\
    & \tilde \vq_i = \vq_i \odot \va_i  \in \R^{d_k}  \quad \tilde \vk_j = \vk_j / \va_j \in \R^{d_k}  \quad \tilde \vv_j = \vv_j \odot \vb_j \in \R^{d_v}  \\
    & \vz_{i} = \textrm{gla}(\vx_{1:i}) = \big( \sum_{j=1}^i \mA_{ij} \vv_j\big) / \vb_i   \in \R^{d_v} \\
    & \text{(rest is the same as the recurrent form)}  \nonumber
\end{align}

$\odot$ and $/$ denotes element-wise multiplication and division; $\sigma$ denotes a sigmoid function.

\paragraph{Connections among Linear Attention, RetNet, GLA} 
RetNet and GLA both inherit the basic linear recurrence with 2-D hidden states from linear attention. GLA and RetNet mainly differ in the decaying term from the perspective of the recurrent form. Specifically, GLA incorporates fine-grained data-dependent gates ($\balpha, \bbeta$) whereas RetNet uses a single fixed decay $\lambda$ that is shared across all tokens and hidden dimensions. The simplicity of decay in RetNet leads to neat attention-style form needed for parallel training. In comparison, GLA's attention-style form is more nuanced, thus resulting in a more complex training schema. Moreover, RetNet and GLA incorporate the additional output gate $\vr_i$ before the output projection $\mW_o$. Such output gating is also used in LSTM and RWKV models presented below.

\subsection[RWKV]{RWKV~\citep{peng2023rwkv}}\label{app:rwkv}
The recurrence of RWKV is motivated by attention-free network \citep{zhai2021attention}, and it uses 1-D hidden state compared with the recurrences of linear attention.  
\begin{align}
    &  \vk_i = \mW_k \vx_i \in \R^{d_v} \quad \vv_i = \mW_v \vx_i  \in \R^{d_v} \\
    & \va_i = \exp(-\vw) \odot \va_{i- 1} + \exp(\vk_i) \odot \vv_i \in \R^{d_v} \\
    & \vb_i = \exp(-\vw) \odot \vb_{i - 1} +  \exp(\vk_i)  \in \R^{d_v} \\
    & \vz_i = \textrm{wkv}(\vx_{1:i}) = \frac{\va_{i-1} + \exp(\vk_i + \vu)\odot \vv_i}{\vb_{i-1} + \exp(\vk_i + \vu)}  \in \R^{d_v} \\
    & \vr_i =  \mW_r\vx_i \in \R^{d_v}  \\
    & \vy_{i} = \mW_o \big( \sigma(\vr_i) \odot \vz_i ) \in \R^{d_v} 
\end{align}
where $\vw, \vu \in \R^{d_v}$ are learnable parameters, $\sigma$ is an activation function. The $\textrm{WKV}$ operators maintain a recurrence with a pair of states ($\va_i, \vb_i$). Different from linear attention where the 2D hidden state is constructed via an outer-product $\vk_i^{\intercal} \vv_i$, $\textrm{WKV}$ uses element-wise dot-product $\exp(\vk_i) \odot \vv_i$, thus the shape of the key and value vectors are the same.

Since the decay term $\vw$ is not data-dependent, $\textrm{WKV}$ also has the following equivalent convolutional form:
\begin{align}
    & \vk_i = \mW_k \vx_i \in \R^{d_v} \quad \vv_i = \mW_v \vx_i  \in \R^{d_v} \\
    & \tilde{\vkv}_i =  \exp(\vk_i) \odot \vv_i \in \R^{d_v}  \quad \tilde \vk_i =  \exp(\vk_i) \in \R^{d_v}  \\
    & \vl_i = \exp(-i\vw)   \in \R^{d_v}  \\
     & \va = \vl \ast \tilde{\vkv} \in \R^{L \times d_v}  \\
     & \vb = \vl \ast \tilde \vk \in \R^{L \times d_v} \\
     & \text{(rest is the same as the recurrent form)}   \nonumber
\end{align}
where $\ast$ denotes batched long convolution operator, i.e., one dimension of the filter $\vh[:, i] \in \R^{L \times 1}$ handles one corresponding dimension $\va[:, i], \vb[:, i] \in \R^{L \times 1}$.
 
\subsection[S4]{S4~\citep{gu2021efficiently}}\label{app:s4}

Structured state space models (S4) is a family of sequence models defined with four parameters $(\Delta, \rmA, \rmB, \rmC)$. S4 is typically represented as a sequence mapping of $\R^{L \times 1} \rightarrow \R^{L \times 1}$, wherein the input and output are both scalars (i.e. $\vx, \vy \in \R^{1}$). In this case, S4 has the following recurrent form.
\begin{align}
&\vh_i = \bar \rmA \vh_{i-1} + \bar \rmB \vx_i \in \R^{d_k} \\ 
&\vy_i = \rmC \vh_i \in \R^{1} 
\end{align}
where $d_{\textrm{inner}}$ denotes the dimension of hidden states $\vh_i$, $\bar \rmA \in \R^{d_{\textrm{inner}} \times d_{\textrm{inner}}}$ and $\bar \rmB \in \R^{d_{\textrm{inner}} \times 1}$ are transformed parameters for discrete sequence data according to a certain discretization rule (e.g., zero-order hold). $\rmC \in \R^{1 \times d_{\textrm{inner}}}$. Equivalently, it has the following convolutional form:
\begin{align}
&\bar \rmK = [\rmC\bar\rmB, \rmC\bar\rmA\bar\rmB, \dots \rmC\bar\rmA^{L-1}\bar\rmB] \\    
&\vy = \vx \ast \bar \rmK
\end{align}
where $\ast$ denotes the convolution operator and $\bar \rmK $ denotes the convolution kernel. The convolution form is critical on enabling efficient parallel training via Fast Fourier Transform (FFT) algorithms.

Since the recurrent forms of other models are usually presented with vector input/output (i.e., $\vx_i, \vy_i \in \R^{d}$), we present its equivalent batched recurrent form as follows:
\begin{align}
    &\rmS_i = \bar \rmA \circ \rmS_{i-1} + \bar \rmB \circ \vx_i \in \R^{d \ \times d_{\textrm{inner}}} \\
    &\vy_i = \rmC \circ \rmS_i  \in \R^{d} \label{eq:s4-batched}
\end{align}
where $\rmS_i$ denotes 2-D hidden states, $\rmA \in \R^{d  \times d_{\textrm{inner}} \times  d_{\textrm{inner}}}, \rmB \in \R^{d \times  d_{\textrm{inner}} \times 1}, \rmC \in \R^{d \times 1 \times d_{\textrm{inner}}}$, $\circ$ denotes batched matrix multiplication.~\footnote{To differentiate the size of hidden states. in recurrences, we use $\vh_i$ in the 1-D cases; $\rmS_i$ in the 2-D cases.} In this batched form, $d$ numbers of independent SSM run in parallel, each responsible for a dimension of input $\vx$.

\paragraph{Connections to Linear Attentions}
With this batched form in \cref{eq:s4-batched}, it becomes clear that S4, similar to linear attention, enjoys a large 2-D hidden states for recurrence. We can also draw a rough parallel between ($\bar \rmB$, $\rmC$) in S4 to ($\vq_i, \vk_j$) in linear attention as they handle the input and output for the recurrences, respectively. The parallel reveals the difference between S4 and linear attention. In S4, the input and output mapping is not data-dependent, i.e., ($\bar \rmB$, $\rmC$) does not depend on input $\vx$. In comparison, $\vq_i$ and $\vk_j$ are linear mappings of the input $\vx_i$. 

\subsection[H3]{H3~\citep{dao2022hungry}} \label{app:h3}
H3 is a mixture of state-space models and linear attention. In particular, it employs the outer-product structure from linear attention (i.e., $\vk_i^T \vv_i$) to construct the input of a state-space model. 
\begin{align}
    & \vk_i = \mW_k \vx_i \in \R^{d_k} \quad \vv_i =  \mW_v\vx_i \in \R^{d_v} \\
    & \vx'_i = \vk_i^\intercal \vv_i \in \R^{d_k \times d_v} \\
    &  \rmS_i = \bar \rmA  \odot \rmS_{i-1} + \bar \rmB \odot\vx'_i  \in \R^{d_k \times d_v \times d_{\text{inner}}} \qquad   \\
    & \vz'_i =  \rmC \circ \rmS_i    \in \R^{d_k \times d_v} \\
    & \vq_i = \mW_q\vx_i  \in \R^{d_k} \\
    & \vz_i = \vq_i \vz'_i \in \R^{d_v} \\
    & \vy_i = \vz'_i \mW_o \in \R^{d} 
\end{align}
where $\bar \rmA$, $\bar \rmB$, $\rmC \in \R^{d_{\textrm{inner}}}$ are parameters of the state-space models, $\odot$ denotes element-wise product with broadcasting, $\circ$ denotes batched matrix-vector product. The SSM is diagonally parameterized (i.e., $\bar \rmA$ is a vector) and the original H3 paper additionally uses another shift-SSM \citep{dao2022hungry} to further refine the key vector $\vk_i$.

\subsection[Hyena]{Hyena~\citep{poli2023hyena}}\label{app:hyena}

Hyena is a pure convolutional model that does not have an equivalent recurrent form, unlike S4. 
However, it recursively applies the convolution operator at the sequence level for $N$ times (i.e., order-$N$ Hyena). In practice, $N$ is usually set to be $2$, and the resulting form is as follows. 

\begin{align}
  & \vv^n = \mW_{n}\vx \in \R^{L \times d} \\
  & \vz^{0}=  \vv^0 \in \R^{L \times d} \\
  & \begin{rcases}
       & \vl^n_i = \operatorname{FFN}(\vi) \in \R^{L \times d} \\
       & \vz^n = \vv^{n-1} \odot (\vl^n  \ast \vz^{n-1}) \in \R^{L \times d} 
  \end{rcases} \text{ recursion } n=1 \dots N \label{eq:hyena-conv} \\
  & \vy = \vz^N \in \R^{L \times d}
\end{align}

where $\ast$ denotes batched convolution operator. In practice, the filter is padded to the size of $(2L - 1) \times d$ so that the convolution operator becomes a circular convolution for efficient training using FFT.~\footnote{Please refer to Section 2 and 3 of \citep{poli2023hyena} for details.}
Note that the resulting kernels $\vl^1, \vl^2$ do not depend on input $\vx$, but the convolution output is controlled by the data-dependent gate $\vv^1, \vv^2$ in \cref{eq:hyena-conv}. %

\subsection[Mamba]{Mamba~\citep{gu2023mamba}}\label{app:mamba}
Mamba has the same recurrent form as S4, and uses data-dependent parameterization for $\bar \rmA$, $\bar \rmB$, $\rmC$:
\begin{align}
    & \vv_i = \mW_v \vx_i  \in \R^{d_v} \\
    & \rmS_i = \bar \rmA_i \odot \rmS_{i-1} + \bar \rmB_i \odot \vv_i \in \R^{d_k \times d_v} \quad (\text{$\odot$ with broadcast}) \\
    & \vy_i =  \rmC_i  \rmS_i \in \R^{d_v} 
\end{align}
where $\bar \rmA_i, \bar \rmB_i \in \R^{d_k \times d_v}$, $\rmC_i \in \R^{d_v}$ data-dependently parameterized, i.e., computed based on $\vx_i/\vv_i$. However, due to the data-dependence, this recurrent form no longer has an equivalent convolutional form for efficient training. The original paper handles this issue with customized hardware-efficient training algorithms based on the recurrent form.
