# Supplementary material for: Learning Syntax Without Planting Trees: Understanding Hierarchical Generalization in Transformers
Source: arXiv:2404.16367 source file (2025-03-16)
Supplement: Supplementary file 5 [file ngram.tex]

\begin{figure}[H]
\begin{python}
def ngram_head(x, hidden_state, shift_step=1, ngram=1):
    """
    Args:
        x: bsz * input_len
        hidden_state: bsz * input_len * d_model
        ngram: 1 means bigram, 2 means trigram
        shift_step: which token to attend to after the matching ngram
    Output:
        bsz * input_len * d_model
    """
    bsz, seq_len = x.shape
    # bsz * L * L, match unigram as the first step
    mask_0 = x[:, None, :] == x[:, :, None]
    causal_mask = torch.tril(torch.ones(seq_len, seq_len, 
        dtype=torch.bool, device=x.device), diagonal=-1 )
    mask_0 = torch.logical_and(mask_0, causal_mask)

    masks = [mask_0.long()]
    for _ in range(1, ngram):
        # mask_0[i, j] = True means token i-1 and token j-1 is matched
        mask_0 = F.pad(mask_0, (1, -1, 1, -1), "constant", False)
        masks.append(mask_0.long())
    ngram_mask = torch.stack(masks, dim=-1).sum(dim=-1) >= ngram
    if shift_step > 0:
        ngram_mask = F.pad(ngram_mask, 
            (shift_step, -shift_step), "constant", False)
    ngram_mask = torch.logical_and(ngram_mask, causal_mask)

    # form a uniform distribution for matched tokens
    ngram_mask_norm = ngram_mask / ngram_mask.sum(dim=2, keepdim=True)
    ngram_mask_norm = torch.nan_to_num(ngram_mask_norm, 0)
    ngram_mask_norm = ngram_mask_norm.to(hidden_state.dtype) 
    output = torch.einsum("bmn,bnz->bmz", ngram_mask_norm, hidden_state)
    return output

class Ngram(nn.Module):
    def __init__(self, d_model, ngram=1):
        super().__init__()
        self.d_model = d_model
        self.ngram = ngram
        self.t0 = nn.Linear(self.d_model, self.d_model)
        self.t1 = nn.Linear(self.d_model, self.d_model)

    def forward(self, x, input_ids):
        bsz, seq_len, _ = x.shape
        h0 = ngram_head(input_ids, x, ngram=self.ngram)
        h1 = x
        y = self.t0(h0) + self.t1(h1)
        return y
\end{python}
\caption{Python implementation of n-gram layers.}
\label{fig:ngramheadcode}
\end{figure}
