# Supplementary material for: Learning Syntax Without Planting Trees: Understanding Hierarchical Generalization in Transformers
Source: arXiv:2404.16367 source file (2025-03-16)
Supplement: Supplementary file 6 [file ngram_module.tex]

\begin{figure}[H]
\begin{python}
class NgramBlock(nn.Module):
    def __init__(self, config, ngram):
        """
        Args:
            ngram: 1, 2, or 3
            
        Note: parameter size 4d^2
        """
        super().__init__()
        self.ln_1 = RMSNorm(config.d_model, eps=1e-5)
        
        self.attn = Ngram(config, ngram)
        self.ln_2 = RMSNorm(config.d_model, eps=1e-5)

        mlp_hidden = config.d_model 
        self.mlp = nn.Sequential(
            nn.Linear(config.d_model, mlp_hidden),
            nn.SiLU(),
            nn.Linear(mlp_hidden, config.d_model),
        )

    def forward(self, x, input_ids):
        x_att = self.attn(self.ln_1(x), input_ids)
        x = x + x_att
        x_mlp = self.mlp(self.ln_2(x))
        x = x + x_mlp
        return x
 
\end{python}
\caption{Python implementation of n-gram blocks with SwiGLU-MLP~\citep{shazeer2020glu} and RMSNorm~\citep{zhang2019root}.}
\label{fig:ngrammodulecode}
\end{figure}
